# Supplementary material for: Sketchy Bounding-box Supervision for 3D Instance Segmentation
Source: arXiv:2505.16399 source file (2025-05-22)
Supplement: Supplementary file 1 [file X_suppl.tex]

%\clearpage
%\setcounter{page}{1}
\maketitlesupplementary
\label{sec:suppl}
This supplementary material provides more details about our method, in which we provide more ablation studies and analysis in Sec.~\ref{sec:suppl_01}, more quantitative and qualitative results in Sec.~\ref{sec:suppl_02}, and
we discuss the limitations and potential applications in Sec.~\ref{sec:suppl_03}.

\section{More ablation studies and analysis}
\label{sec:suppl_01}
\textbf{Number of the query vectors.} Since the performances of the query-based methods are sensitive to the predefined number of the query vectors, following existing methods \cite{schult2023mask3d, sun2023superpoint}, we conducted the ablation studies on the number of the query vectors. Table~\ref{tab:tab10} presents the experimental results of various numbered query vectors on the ScanNetV2 validation set. It can be observed that the performance improved nearly as the increasing of the number of the query vectors, and our method obtains considerable performance at the number of the query vectors $Q=400$, when the number is equal to 600, the performance degrades. Thus we set $Q=400$ in our final experiments.

\textbf{Number of the multi-level attention blocks.}
We implement an ablation experiment about the block number of the Multi-level Attention Block. As shown in Table~\ref{tab:tab15}, the best performance is achieved when the block number is set as 6.

\textbf{Ablation study about the hyper-parameter $\lambda$.}
We perform the ablation experiment about the loss weights of coarse-to-fine instance segmentator in Table~\ref{tab:tab16}, and it can be observed that the best performance is achieved when the $\lambda_1$, $\lambda_2$, $\lambda_3$ are set as $0.5$, $1.0$, $0.5$, respectively.

\textbf{Efficiency of the model training.} In Fig. \ref{fig:figure07}, we make a qualitative comparison between GaPro \cite{ngo2023gapro} and our method, which both utilize the same training strategy as SPFormer \cite{sun2023superpoint}. On the one hand, it can be observed that our model converges quicker in the first 200 epochs, which illustrates that our method can converge at a higher speed. On the other hand, our method trained for 400 epochs while the GaPro is trained for 512 epochs in total, which verifies that our method requires less training cost. 

\textbf{Effectiveness of the multi-level attention blocks.} In Fig. \ref{fig:figure11}, we compare the visualization of instance segmentation results on the ScanNetV2 validation set. The coarse instances are the visualization of the initially predicted instances of the coarse-to-fine instance segmentator, while the fine instances are the corresponding visualization after deploying the multi-level attention blocks. It can be observed that without the multi-level attention blocks, the unreliable region of the table can not be segmented precisely (illustrated both in the 1st and 2nd rows), and the chairs closely can not be differed (illustrated in the 3rd row). With the multi-level attention blocks, the segmented objects are refined, and our model obtains well-detailed instances, which verifies that our proposed multi-level attention blocks can segment instances in a coarse-to-fine manner.

\begin{table}
  \caption{\textbf{Ablation Study of the number of the query vectors} using accurate bounding boxes.}
  \label{tab:tab10}
  \centering
  \setlength{\tabcolsep}{8mm}
  \begin{tabular}{@{}lccc@{}@{}@{}}
    \toprule
    Number & $AP$ & $AP_{50}$ & $AP_{25}$ \\
    \midrule
    %100 & 37.0 & 57.7 & 74.9 \\
    200 & 43.7 & 66.4 & 82.4 \\
    %300 & 40.0 & 61.0 & 76.7 \\
    400 & \textbf{46.0} & \textbf{68.8} & \textbf{83.6} \\
    %500 & 38.1 & 58.9 & 74.8 \\
    600 & 45.6 & 68.1 & 83.5 \\
    \bottomrule
  \end{tabular}
\end{table}

\begin{table}
  \caption{\textbf{Ablation Study of the number of the multi-level attention blocks} using $S_{4}$ sketchy bounding boxes.}
  \label{tab:tab15}
  \centering
  \setlength{\tabcolsep}{13.8mm}
  \begin{tabular}{@{}lcc@{}@{}}
    \toprule
    Number & $AP_{50}$ & $AP_{25}$ \\
    \midrule
    2 & 60.6 & 77.4 \\
    4 & 61.9 & 76.7 \\
    6 & \textbf{62.5} & \textbf{80.1} \\
    8 & 60.2 & 76.4 \\
    \bottomrule
  \end{tabular}
\end{table}

\begin{table}
  \caption{\textbf{Ablation study about the hyper-parameter $\lambda$} for the instance segmentation loss using $S_{4}$ sketchy bounding boxes.}
  \label{tab:tab16}
  \centering
  \setlength{\tabcolsep}{6.6mm}
  \begin{tabular}{@{}lcccc@{}@{}@{}@{}}
    \toprule
    $\lambda_1$ & $\lambda_2$ & $\lambda_3$ & $AP_{50}$ & $AP_{25}$ \\
    \midrule
    0.1 & 1.0 & 0.5 & 38.3 & 46.1 \\
    0.5 & 0.5 & 0.5 & 57.1 & 74.7 \\
    0.5 & 1.5 & 0.5 & 59.7 & 75.1 \\
    0.5 & 1.0 & 1.0 & 58.6 & 74.1 \\
    0.5 & 1.0 & 1.5 & 54.9 & 70.5 \\
    0.5 & 1.0 & 0.5 & \textbf{62.5} & \textbf{80.1} \\
    \bottomrule
  \end{tabular}
\end{table}

\section{More quantitative and qualitative results}
\label{sec:suppl_02}
\textbf{Results of 3D object detection.} The instance predictions can be transformed into bounding box predictions by obtaining the two corner coordinates of the predicted binary masks.
in Table \ref{tab:tab11}, we compare the object detection result with the state-of-the-art 3D object detection methods \cite{qi2019deep, xie2020mlcvnet,misra2021end, zhang2020h3dnet, liu2021group, wang2022rbgnet, zheng2022hyperdet3d, rukhovich2022fcaf3d, wang2022cagroup3d} and 3D instance segmentation methods \cite{schult2023mask3d, lai2023mask}. 
And the leading performance of our method on the 3D object detection task has further verified that our designed Sketchy-3DIS can explore the underlying instance characteristics indicated by the bounding boxes.

\textbf{Quantity comparisons of pseudo labels on ScanNetV2 training set.} We compare the quality of the pseudo labels of the GaPro \cite{ngo2023gapro} and our method. The experimental results are shown in Table \ref{tab:tab14}, the per-category results of $AP_{50}$ indicate that our method can generate more accurate pseudo labels than GaPro. 

\textbf{Comparison of parameters and training time. } In Table \ref{tab:tab09}, we compare the training time and parameters of the pseudo labeling task and instance segmentation task on GaPro \cite{ngo2023gapro}, BSNet \cite{lu2024bsnet} and ours Sketchy-3DIS. Compared with these two state-of-the-art approaches, our method requires less training time and parameters, especially on the ScanNetV2 dataset, which verifies that our method can achieve the box-supervised 3D instance segmentation efficiently and economically.

\textbf{Visualization of predicted instances on the ScanNetV2 test set. } In Fig. \ref{fig:figure09}, we present some samples of predicted instances on the ScanNetV2 test set, in which we utilize various colors to represent different objects. For an input point cloud, our proposed Sketchy-3DIS can correctly segment each instance and produce well-detailed segmentation results. 

\begin{table}
\caption{\textbf{3D Object detection results on the ScanNetV2 validation set.}}
\label{tab:tab11}
  \centering
  \setlength{\tabcolsep}{0.5mm}
  \begin{tabular}{@{}lccc@{}@{}@{}}
    \toprule
    Method & Task & $Box\_AP_{50}$ & $Box\_AP_{25}$ \\
    \midrule
    VoteNet \cite{qi2019deep} & \multirow{9}*{Detection} & 33.5 & 58.6 \\
    MLCVNet \cite{xie2020mlcvnet} & ~ & 41.4 & 64.5 \\
    3DETR \cite{misra2021end} & ~ & 47.0 & 65.0 \\
    H3DNet \cite{zhang2020h3dnet} & ~ & 48.1 & 67.2 \\
    Group-free \cite{liu2021group} & ~ & 52.8 & 69.1 \\
    RBGNet \cite{wang2022rbgnet} & ~ & 55.2 & 70.6 \\
    HyperDet3D \cite{zheng2022hyperdet3d} & ~ & 57.2 & 70.9 \\
    FCAF3D \cite{rukhovich2022fcaf3d} & ~ & 57.3 & 71.5 \\
    CAGroup3D \cite{wang2022cagroup3d} & ~ & \textbf{61.3} & \textbf{75.1} \\
    \midrule
    Mask3D \cite{schult2023mask3d} & \multirow{3}*{Segmentation} & 56.2 & 70.2 \\
    MAFT \cite{lai2023mask} & ~ & 63.9 & 73.5 \\
    Sketchy-3DIS (ours) & ~ & \textbf{64.0 (+2.7)} & \textbf{79.4 (+4.3)} \\
    \bottomrule
  \end{tabular}
\end{table}

\begin{table}
  \caption{\textbf{Comparison of parameters and training time.} The parameters and training time are the total statistics for pseudo labeling and instance segmentation. }
  \label{tab:tab09}
  \centering
  \setlength{\tabcolsep}{2.9mm}
  \begin{tabular}{@{}lccc@{}@{}@{}}
    \toprule
    Method & Dataset & T (h) & P (M) \\
    \midrule
    GaPro \cite{ngo2023gapro} + SPFormer & \multirow{3}*{ScanNetV2} & 80 & 17.6 \\
    BSNet \cite{lu2024bsnet} + SPFormer & ~ & 37 & 20 \\
    Sketchy-3DIS (ours) & ~ & \textbf{23} & \textbf{14.2} \\
    \midrule
    GaPro \cite{ngo2023gapro} + ISBNet & \multirow{3}*{S3DIS} & 150 & 31.1 \\
    BSNet \cite{lu2024bsnet} + ISBNet & ~ & 72 & 33.1 \\
    Sketchy-3DIS (ours) & ~ & \textbf{59} & \textbf{30.7} \\
    \bottomrule
  \end{tabular}
\end{table}

\textbf{Per-category instance segmentation results.} We show per-category instance segmentation results on ScanNetV2 validation set and test set in Table \ref{tab:tab12} and Table \ref{tab:tab13}, respectively. It can be observed that our method achieves considerable performance on both the ScanNetV2 validation set and the test set.

\begin{figure*}[t]
  \centering
   \includegraphics[width=0.98\linewidth]{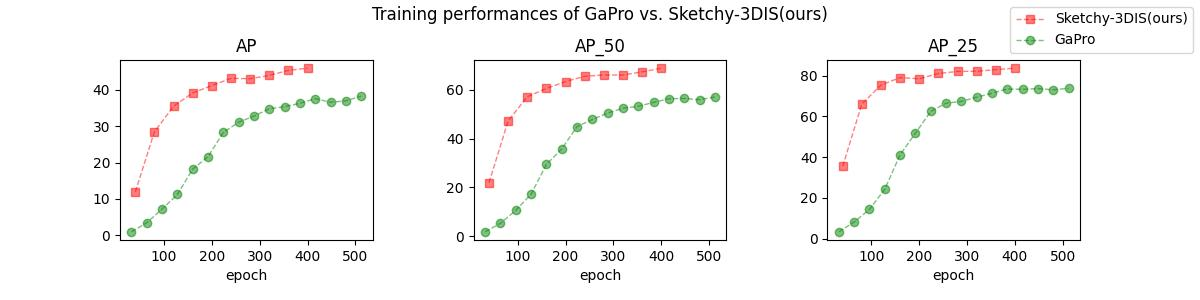}
   \vspace{-1.0em}
   \caption{\textbf{Efficiency of the model training.} The figure compares the performance of GaPro \cite{ngo2023gapro} and ours Sketchy-3DIS during the training process on the ScanNetV2 validation set. }
   \label{fig:figure07}
\end{figure*}

\begin{table*}
  \caption{\textbf{Quality of pseudo labels on ScanNet v2 training set.} The comparisons in $AP_{50}$ of each object category is shown in this table.}
  
  \label{tab:tab14}
  \centering
  \setlength{\tabcolsep}{1mm}{
      \resizebox{\textwidth}{16mm}{
      \begin{tabular}{@{}lccccccccccccccccccc@{}@{}@{}@{}@{}@{}@{}@{}@{}@{}@{}@{}@{}@{}@{}@{}@{}}
        \toprule
        \rule{0pt}{13pt}
        \small Method & \small $AP_{50}$ & \rotatebox{90}
        {\small bath} & \rotatebox{90}{\small bed} & \rotatebox{90}{\small bkshf} & \rotatebox{90}{\small cabinet} & \rotatebox{90}{\small chair} & \rotatebox{90}{\small counter} & \rotatebox{90}{\small curtain} & \rotatebox{90}{\small desk} & \rotatebox{90}{\small door} & \rotatebox{90}{\small other fur.} & \rotatebox{90}{\small picture} & \rotatebox{90}{\small fridge} & \rotatebox{90}{\small s. cur.} & \rotatebox{90}{\small sink} & \rotatebox{90}{\small sofa} & \rotatebox{90}{\small table} & \rotatebox{90}{\small toilet} & \rotatebox{90}{\small window} \\
        \midrule
        \rule{0pt}{10pt} 
        GaPro \cite{ngo2023gapro} & 81.9 & 99.1 & 85.9 & 82.4 & 88.2 & 74.8 & 48.9 & 74.5 & 45.6 & 81.0 & 84.4 & 95.6 & 88.4 & 94.9 & 87.0 & 91.3 & 72.2 & 92.7 & 88.0 \\
        \rule{0pt}{10pt} 
        Sketchy-3DIS (ours) & \textbf{86.8} & 97.1 & 85.5 & 84.0 & 87.6 & 96.0 & 48.6 & 89.8 & 59.3 & 81.1 & 94.2 & 85.7 & 96.5 & 98.4 & 90.2 & 97.3 & 85.1 & 99.5 & 85.7 \\
        \bottomrule
      \end{tabular}
      }
  }
\end{table*}

\section{The limitations and potential applications}
\label{sec:suppl_03}
\textbf{Limitations.} The proposed Sketchy-3DIS is a bounding-box supervised method that tolerates the inaccurate annotated boxes, however, the performance would suffer degradation once the annotated boxes are with huge inaccuracy. Additionally, the bounding-box annotations obtained from the point-wise annotations of the input point cloud is limited, which are the same as the existing methods \cite{ngo2023gapro, chibane2022box2mask, du2023weakly}. Last but not least, the related datasets \cite{dai2017scannet, armeni20163d} are preprocessed and aim for academic research, there may be some variations in real situations.

\begin{table*}
  \caption{\textbf{Per-category instance segmentation results of Sketchy-3DIS (ours) on ScanNetV2 validation set.} For reference purposes, we show the results of instance segmentation results on ScanNetV2 validation set.}
  \label{tab:tab12}
  \centering
  \setlength{\tabcolsep}{3.9mm}
  \begin{tabular}{@{}lccccccccc@{}@{}@{}@{}@{}@{}@{}@{}@{}}
    \toprule
     & bath & bed & bookshelf & cabinet & chair & counter & curtain & desk & door \\
    \midrule
    $AP$ & 75.1 & 23.4 & 29.5 & 39.3 & 76.5 & 15.5 & 41.0 & 9.4 & 46.3 \\
    $AP_{50}$ & 87.3 & 60.3 & 61.4 & 64.7 & 94.0 & 48.4 & 68.6 & 36.8 & 69.8 \\
    $AP_{25}$ & 87.3 & 60.3 & 61.4 & 64.7 & 94.0 & 48.4 & 68.6 & 36.8 & 69.8 \\
    \midrule
    & other fur. & picture & fridge & s. cur. & sink & sofa & table & toilet & window \\
    \midrule
    $AP$ & 53.9 & 51.9 & 50.0 & 51.2 & 51.9 & 50.9 & 40.7 & 87.4 & 34.8 \\
    $AP_{50}$ & 69.2 & 67.7 & 68.7 & 70.2 & 73.7 & 78.1 & 66.7 & 94.7 & 57.7 \\
    $AP_{25}$ & 77.4 & 77.0 & 73.0 & 83.7 & 91.9 & 90.5 & 85.0 & 99.4 & 75.6 \\
    \bottomrule
  \end{tabular}
\end{table*}

\begin{table*}
  \caption{\textbf{Per-category instance segmentation results of Sketchy-3DIS (ours) on ScanNetV2 test set.} For reference purposes, we show the results of instance segmentation results on ScanNetV2 test set.}
  \label{tab:tab13}
  \centering
  \setlength{\tabcolsep}{3.9mm}
  \begin{tabular}{@{}lccccccccc@{}@{}@{}@{}@{}@{}@{}@{}@{}}
    \toprule
     & bath & bed & bookshelf & cabinet & chair & counter & curtain & desk & door \\
    \midrule
    $AP$ & 74.1 & 32.0 & 31.0 & 37.1 & 70.4 & 5.7 & 39.0 & 11.6 & 41.0 \\
    $AP_{50}$ & 100.0 & 72.0 & 66.7 & 67.0 & 87.7 & 12.3 & 69.1 & 43.9 & 69.7 \\
    $AP_{25}$ & 100.0 & 95.5 & 76.1 & 80.5 & 95.0 & 78.5 & 75.7 & 91.3 & 90.8 \\
    \midrule
    & other fur. & picture & fridge & s. cur.& sink & sofa & table & toilet & window \\
    \midrule
    $AP$ & 47.9 & 60.2 & 52.0 & 67.1 & 48.9 & 58.0 & 37.3 & 85.0 & 38.4 \\
    $AP_{50}$ & 62.7 & 67.0 & 64.5 & 100.0 & 80.7 & 77.6 & 60.3 & 100.0 & 60.4 \\
    $AP_{25}$ & 73.7 & 80.0 & 73.5 & 100.0 & 91.1 & 94.9 & 81.8 & 100.0 & 80.7 \\
    \bottomrule
  \end{tabular}
\end{table*}

\textbf{Potential applications.} The proposed Sketchy-3DIS can be applied as a pre-annotation strategy for tasks that require dense-level annotations. Moreover, this work can facilitate the development of some applications of robotics and autonomous driving, in which the navigation system can obtain the objective signals benefit by the high performance on $AP_{25}$ of our proposed Sketchy-3DIS.

\textbf{Future work.} In the future, we will consider adapting our method to dynamic situations to make full use of the robustness characteristic of our proposed Sketchy-3DIS. We also consider expanding our method to a wide range of tasks such as the few-shot instance segmentation, object detection, and part segmentation.

\begin{figure*}[t]
  \centering
   \includegraphics[width=0.98\linewidth]{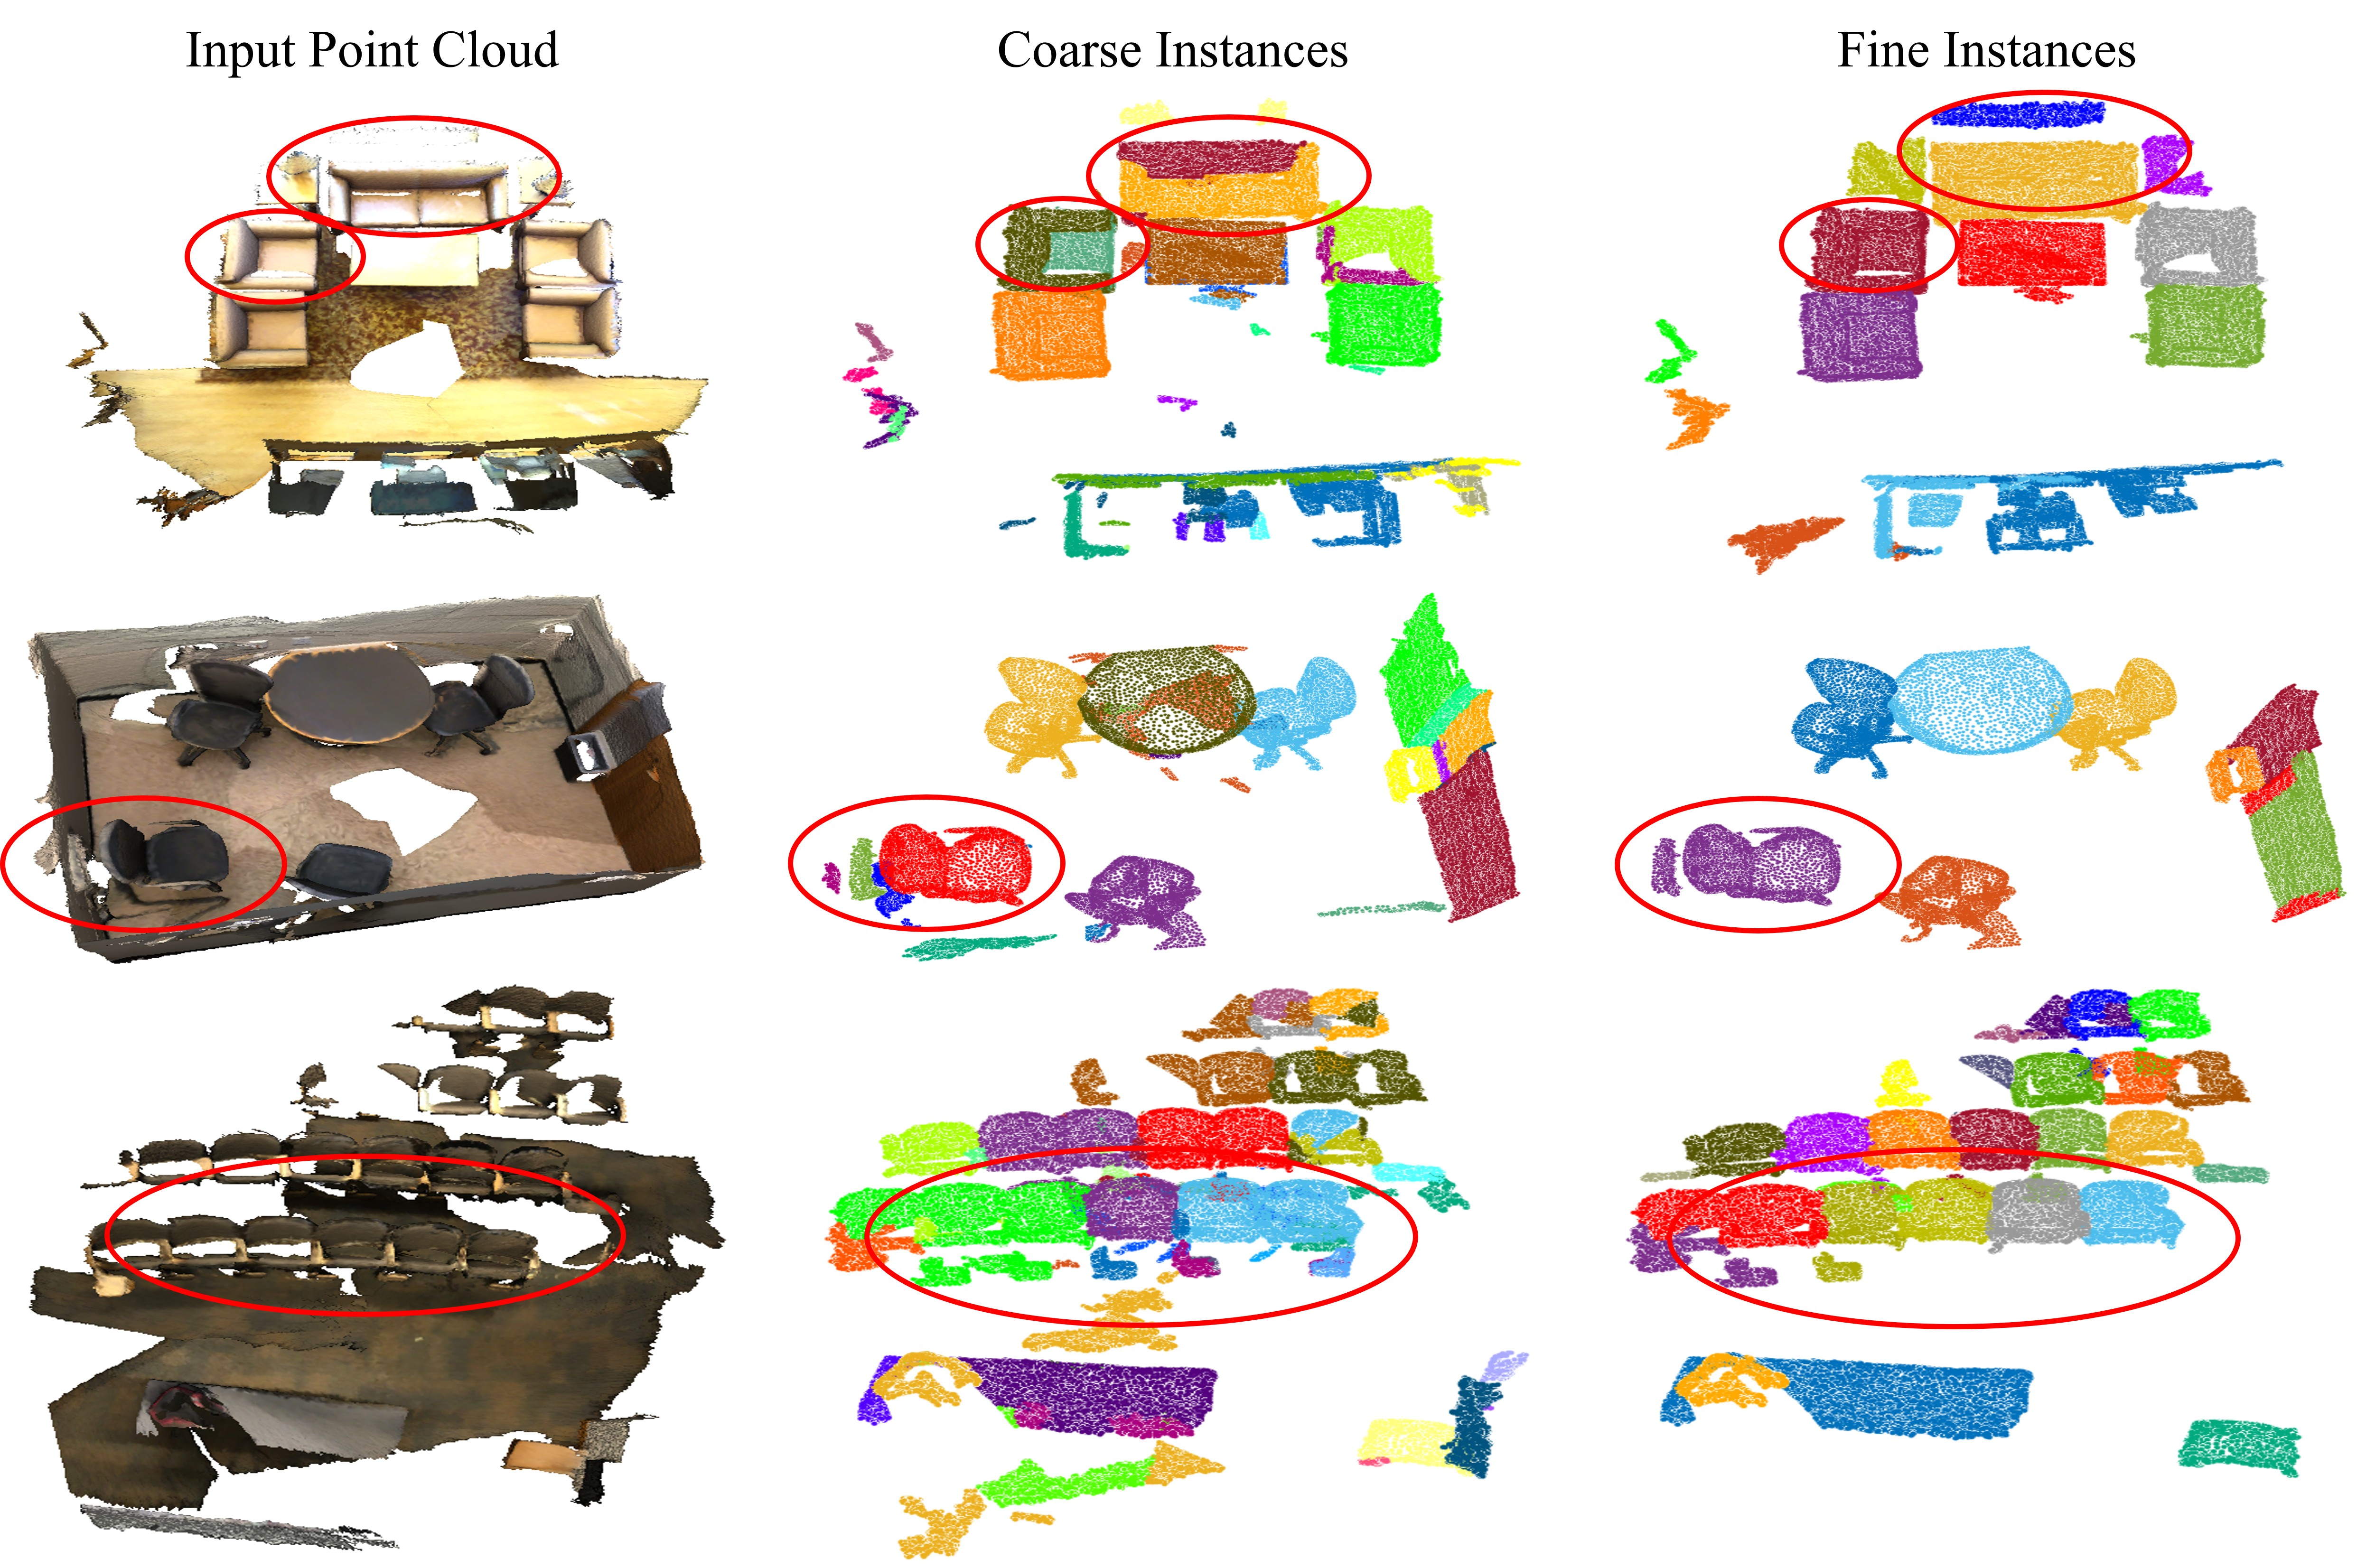}
   \caption{\textbf{Effectiveness of the Multi-level Attention Block.} ``Coarse Instances'' illustrate the predicted instances before the multi-level attention blocks in the coarse-to-fine instance segmentator, while ``Fine Instances'' illustrate the fine instances obtained after deploying the multi-level attention blocks. The red cycles highlight the key objects.}
   \label{fig:figure11}
\end{figure*}

\begin{figure*}[t]
  \centering
   \includegraphics[width=1.0\linewidth]{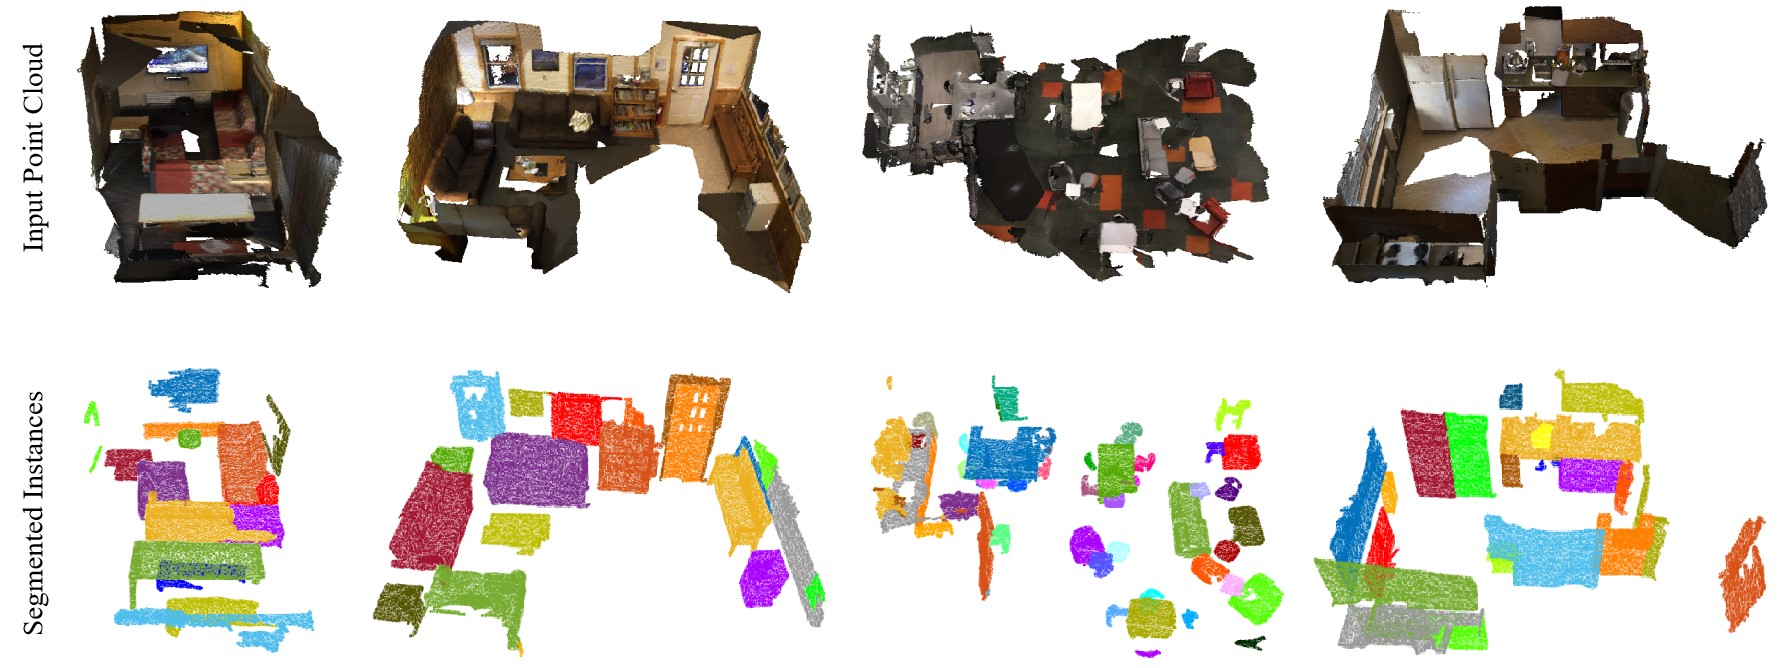}
\caption{\textbf{Qualitative results on ScanNetV2 test set.} The top row denotes the input point cloud and the bottom row denotes the corresponding segmented instances. }
   \label{fig:figure09}
\end{figure*}
